# Supplementary material for: Efficient Sample-optimal Learning of Gaussian Tree Models via Sample-optimal Testing of Gaussian Mutual Information
Source: arXiv:2411.11516 source file (2024-11-18)
Supplement: Supplementary file 1 [file prelim_appendix.tex]

\section{Additional preliminaries}\label{sec:prelim_app}

%In this section, we introduce several definitions that will be used in our proofs.

Now we introduce several definitions that will be used in our proofs. Let us start with the notion of sub-exponential random variables.

\begin{defi}[Sub-exponential random variable]
A random variable $X$ is said to be \emph{sub-exponential} if the moment generating function of $\abs{X}$ satisfies:
\[
\E [\exp\paren{|X|/{K}}] \le 2,
\]
for some $K$. The smallest such $K$ is called the sub-exponential norm of $X$, denoted $\abs{\abs{X}}_{\psi}$.
\end{defi}

\begin{fact}\label{fact:sqgauss}
    Let $g\sim N(0,1)$  be a standard Gaussian random variable. Then $\abs{\abs{g^2}}_{\psi}\le \frac{8}{3}$.
\end{fact}

\begin{lem}[Bernstein inequality, Theorem $2.8.1$ of \cite{vershynin2018high}]\label{lem:bernsteain}
Let $X_1, \ldots, X_N$ be $N$ independent zero-mean sub-exponential random variable $X$. Then there exists an absolute constant $c>0$ such that for every $t\ge 0$
\[
\mathrm{Pr}\left[
\sum_{i=1}^N X_i\ge t
\right] \le 2\exp\left[
-c\cdot \min\paren{
\frac{t^2}{\sum_{i} \abs{\abs{X_i}}_{\psi}^2},
\frac{t}{\max_i \abs{\abs{X_i}}_{\psi}}
}
\right]
\]

\end{lem}

Let $T$ be an undirected tree on the vertex set $[n]$. Consider a vertex $i \in [n]$ as the root of $T$. Then the rooted orientation of $T$ orients the edges from the root $i$. Given a node $i$, $pa(i)$ denotes the parent node of $i$, or null if $i$ is the root node, and $nd(i)$ denotes the set of vertices not reachable from $i$.

% \begin{defi}[Tree-structured distribution]
% Let $T$ be a tree on the vertex set $[n]$, and consider a rooted-orientation of $T$, and order the nodes of $T$ in the topological order. A distribution $P$ over $X=(X_1, \ldots,X_n) \in \R^n$ is said to be a $T$-structured distribution if every variable $X_i$ is conditionally independent of $\{X_j : j \in nd(i)\}$ given $X_{pa(i)}$. Moreover, $P$ has the following factorization:
% \color{red}
% $$\Pr[X=x]:= \Pr[X_1=x_1] \cdot \prod \Pr[X_i=x_i \mid X_{pa(i)}=x_{pa(i)}]$$
% \color{black}
% A distribution $P$ is said to be tree-structured if it is $T$-structured for some tree $T$.
% \end{defi}

\begin{lem}\label{lem:treeci}[\cite{verma2022equivalence}]
Let us consider a tree $T$ with the vertex set $[n]$. Moreover, consider a $T$-structured distribution $P$ on $(X_1, \ldots,X_n)$. For any three nodes $i,j,k \in [n]$, if the path from $i$ to $k$ passes through $j$ in $T$, then  $X_i$ and $X_k$ are conditionally independent given $X_j$.
\end{lem}

\begin{lem}[\cite{bhattacharyya2023near}]\label{lem:spanningtreelemma}
Let $T_1$ and $T_2$ be two spanning trees on the vertex set $[n]$. Consider the symmetric difference of $T_1$ and $T_2$: $F=\{f_1, \ldots, f_{\ell}\}$ and $G=\{g_1, \ldots,g_{\ell}\}$. Then $F$ and $G$ can be paired up, say $\langle f_i, g_i \rangle$ such that $T_1 \cup \{f_i\} \setminus \{g_i\}$ is a spanning tree for all $i \in [\ell]$.   
\end{lem}

% \begin{defi}[KL-divergence between two distributions]
% Let $P$ and $Q$ be two distributions defined over $\R^n$. Then the $KL$-divergence between $P$ and $Q$ is defined as follows: 
% $$\kl(P||Q)= \int_{x \in \R^n} P(x) \log \frac{P(x)}{Q(x)} dx$$
% \end{defi}

% \begin{defi}[Hellinger distance between two distributions]
% Let $P$ and $Q$ be two distributions defined over $\R^n$. Then the squared-Hellinger distance between $P$ and $Q$ is defined as follows: 
% $$H^2(P,Q)= \int_{x \in \R^n} \frac{1}{2} \cdot \left(\sqrt{P(x)}-\sqrt{Q(x)}\right)^2 dx$$ 
% \end{defi}

\begin{defi}[Total variation distance]
Let $P$ and $Q$ be two probability distributions over $\R^n$ with density functions $P$ and $Q$. The total variation distance between $P$ and $Q$ is:
$$\mathsf{d_{TV}}(P,Q)=\frac{1}{2}\int_{\R^n}|dP-dQ|$$
%\ssnotes{would it be dP and dQ?}\sgnotes{I think it's fine. dP and dQ are differentials of the functions P and Q.}
%$$\mathsf{d_{TV}}(P,Q)=\frac{1}{2}\int_{\R^n}|P-Q| dx$$  
\end{defi}

%\ssnotes{do we need to define dP and dQ?}

% \begin{defi}[Total variation distance]
% Let $P$ and $Q$ be two probability distributions over $\R^n$. The total variation distance between $P$ and $Q$ is defined as follows:
% $$\mathsf{d_{TV}}(P,Q)=\frac{1}{2}\int_{\R^n}|P-Q| dx$$  
% \end{defi}

\begin{lem}[Pinkser's inequality]\label{lem:pinkser}
Let $P$ and $Q$ be two probability distributions. Then the following holds:
$$\mathsf{d_{TV}}(P,Q) \leq \sqrt{\frac{\kl(P||Q)}{2}}$$
\end{lem}

\begin{obs}\label{obs:klhellingerbounds}
Let $P$ and $Q$ be two zero-mean Gaussian distributions such that $P \sim N(0, \Sigma_1)$ and $Q \sim N(0,\Sigma_2)$. Then the $KL$-divergence between $P$ and $Q$ can be expressed as follow~\citep[Page 13]{duchi2007derivations}:
    \begin{equation}
     \kl(P || Q) = \frac{1}{2} \left(\tr(\Sigma_2^{-1} \Sigma_1) - \mathsf{dim}(\Sigma_1) + \ln\left(\frac{\det(\Sigma_2)}{\det(\Sigma_1)}\right)\right)   
    \end{equation}

% Then we have the following:

% \begin{itemize}
%     \item[(i)] The $KL$-divergence between $P$ and $Q$ can be expressed as follow~\citep[Page 13]{duchi2007derivations}:
%     \begin{equation}
%      \kl(P || Q) = \frac{1}{2} \left(tr(\Sigma_2^{-1} \Sigma_1) - \mathsf{dim}(\Sigma_1) + \ln\left(\frac{\det(\Sigma_2)}{\det(\Sigma_1)}\right)\right)   
%     \end{equation}

%     \item[(ii)] The squared-Hellinger distance between $P$ and $Q$ can be expressed as follows~\citep[Page 51]{pardo2018statistical}:
%     \begin{equation}
%         H^2(R_1,R_2)= 1- \frac{\det(\Sigma_1)^{1/4} \cdot \det(\Sigma_2)^{1/4}}{\det(\frac{\Sigma_1 + \Sigma_2}{2})^{1/2}}
%     \end{equation}
% \end{itemize}

\end{obs}

\begin{obs}[Folklore, see \citep{kelner2020learning}]\label{obs:empcovmatrixbound}
Let $P$ be an unknown zero-mean Gaussian distribution defined over $\R^n$ and let $\eps, \delta \in (0,1)$ be two parameters. Given $m$ i.i.d. random vectors $X^{(1)}, \ldots, X^{(m)}$ from $P$, let $\widehat{\Sigma}$ be the empirical covariance matrix. Then if {$m=\Oh\paren{\paren{n+\log \delta^{-1}}\eps^{-2}}$} with probability at least $1-\delta$, the following holds:
$$(1-\eps)\Sigma \preceq \widehat{\Sigma} \preceq (1+\eps)\Sigma$$
\end{obs}

%\ssnotes{the bound in the red part: is it additive or multiplicative? i think its additive, right?}

% \begin{proof}
% In order to prove the above, 

% We will use the following result from \citep[Lemma 11]{kelner2020learning}.

% \begin{lem}\label{lem:covmatrixbound}
% Let $P$ be an unknown distribution defined over $\R^n$. Suppose $\eps \in (0, \frac{1}{2})$ and $\delta > 0$. Then, for any $m$ such that $\eps \geq C_1 (\sqrt{\frac{n}{m}} + \sqrt{\frac{\log(2/\delta)}{m}})$ and $X^{(1)}, \ldots, X^{(m)}$, with probability at least $1-\delta$, we have that 
% $$(1-\eps)\Sigma \preceq \frac{1}{m} \sum_{i=1}^m X^{(i)}(X^{(i)})^T \preceq (1+\eps)\Sigma.$$    
% \end{lem}

% \begin{lem}[Fano's inequality]
    
% \end{lem}

\begin{lem}[Le Cam's two point method: \cite{yu1997cam}]\label{lem:lecam}
    Let $P$ and $Q$ be two distributions. Given a random unknown distribution $R\in \{P,Q\}$, any algorithm that takes a single sample from $R$ will be incorrect with at least $\paren{\frac{1}{2}-\frac{\mathsf{d_{TV}}(P,Q)}{2}}$ probability in guessing $R$.
\end{lem}
